# Supplementary material for: What Drives Online Popularity: Author, Content or Sharers? Estimating Spread Dynamics with Bayesian Mixture Hawkes
Source: arXiv:2406.03390 source file (2024-08-21)
Supplement: Supplementary file 1 [file supplementary.pdf]

# Supplementary Material for *What Drives Online Popularity: Author, Content or Sharers? Estimating Spread Dynamics with Bayesian Mixture Hawkes*

Pio Calderon<sup>(✉)</sup>[0000-0002-8747-8917] and Marian-Andrei  
Rizoiu<sup>[0000-0003-0381-669X]</sup>

University of Technology Sydney, Australia  
piogabrielle.b.calderon@student.uts.edu.au  
marian-andrei.rizoiu@uts.edu.au

## 1 Background Material

### 1.1 Hawkes Process

**Inference.** Given a cascade  $\mathcal{H}$  of length  $N$ , i.e. an ordered collection of time stamps  $\{t_i\}_{i=1}^N$  observed until some terminal time  $T \geq t_N$ , we can estimate the parameters of the Hawkes process  $(\mu^*, \alpha^*, \boldsymbol{\Theta}^*)$  that generated the data by maximizing the log-likelihood function,

$$\mathcal{L}(\mu, \alpha, \boldsymbol{\Theta} | \mathcal{H} = \{t_j\}_{j=1}^N) = \sum_{j=1}^N \log \lambda(t_j; \mu, \alpha, \boldsymbol{\Theta}) - \int_0^T \lambda(s; \mu, \alpha, \boldsymbol{\Theta}) ds. \quad (1)$$

This approach can be extended to the case of a collection of cascades  $\mathbb{H} = \{\mathcal{H}_i\}$ , where the best-fitting Hawkes process is obtained by maximizing the sum of the log-likelihood functions,

$$\mathcal{L}(\mu, \alpha, \boldsymbol{\Theta} | \mathbb{H}) = \sum_{\mathcal{H}_i \in \mathbb{H}} \mathcal{L}(\mu, \alpha, \boldsymbol{\Theta} | \mathcal{H}_i). \quad (2)$$

**Prediction.** The fitted Hawkes process can be leveraged to predict the cascade size  $\hat{N}$  of a new cascade  $\mathcal{H} \in \mathbb{H}$ :

$$\hat{N} = \mathbb{E}[N | \alpha] = \text{logit}(\alpha). \quad (3)$$

### 1.2 Dual Mixture Model

**Inference.** Given the pre-defined number of components  $K$ , we obtain the Borel mixture model  $M^B$  by maximizing the following log-likelihood function,

$$\mathcal{L}_{BMM} = \sum_{\mathcal{H}_i \in \mathbb{H}} \log \sum_{k=1}^K p_k^B \mathbb{B}(N_i | \alpha_k^*). \quad (4)$$

Note that the DMM is not formulated as a Bayesian model in [2] and the Expectation-Maximization (EM) algorithm [4] is employed to maximize  $\mathcal{L}_{BMM}$ . Similarly, the kernel mixture model  $M^g$  is obtained by applying the EM algorithm to the kernel log-likelihood

$$\mathcal{L}_{KMM} = \sum_{\mathcal{H}_i \in \mathbb{H}} \log \sum_{k=1}^K p_k^g f^g(\mathcal{H}_i | \Theta_k^*), \quad (5)$$

where  $f(\mathcal{H}_i | \Theta) = \prod_{t_j \in \mathcal{H}_i} \sum_{t_z < t_j} g(t_j - t_z | \Theta)$ .

**Cold Start Popularity Prediction.** Assume that we are given a collection of related cascade groups  $\{\mathbb{H}_a\}_{a \in \mathcal{A}}$ . For instance, suppose  $\mathcal{A}$  is a set of news articles from a common online publisher  $\rho$  and  $\mathbb{H}_a$  is the set of retweet cascades discussing article  $a$ . Give a yet-to-be-published article  $a^* \notin \mathcal{A}$ , we wish to model its popularity  $\hat{N}^{a^*}$  by learning from historical data  $\{\mathbb{H}_a\}_{a \in \mathcal{A}}$ .

To do this, we can construct a publisher-level popularity model  $M_\rho^B$  by fitting an independent BMM  $M_a^B$  (with  $K_a$  classes) to each  $\mathbb{H}_a$  and then collecting these as a mixture  $M_\rho^B$  over  $\mathcal{A}$ , i.e.,

$$M_\rho^B = \bigcup_{a \in \mathcal{A}} M_a^B = \bigcup_{a \in \mathcal{A}} \left\{ \left( \alpha_1^a, \frac{p_1^{B,a}}{|\mathcal{A}|} \right), \dots, \left( \alpha_{K_a}^a, \frac{p_{K_a}^{B,a}}{|\mathcal{A}|} \right) \right\}, \quad (6)$$

where  $(\alpha_i^a, p_i^{B,a}) \in M_a^B$ . We can estimate the cold-start popularity of a new article  $a^*$  as

$$\hat{N}^{a^*} = \hat{C}_\rho \cdot \mathbb{E}_{M_\rho^B} [\text{logit}(\alpha)] = \hat{C}_\rho \cdot \sum_{a \in \mathcal{A}} \sum_{i=1}^{K_a} \text{logit}(\alpha_i^a) \cdot \frac{p_i^{B,a}}{|\mathcal{A}|}, \quad (7)$$

where  $\hat{C}_\rho$  is an estimate of the cascade count of article  $a^*$ , which we can take as the average cascade count of articles in  $\mathcal{A}$ .

### 1.3 Bayesian Hierarchical Modeling

Let  $\theta$  be a parameter set of a generative process  $\mathcal{P}$  and  $\mathcal{D}$  be a sample from  $\mathcal{P}$ . Bayesian inference involves (1) quantifying our prior belief on  $\theta$  through a prior distribution  $\mathbb{P}(\theta)$ , which could be uninformative or based on expert opinion, and then (2) updating  $\mathbb{P}(\theta)$  using the data  $\mathcal{D}$ , with the likelihood function  $\mathcal{L}(\mathcal{D} | \theta)$  serving as our weight on  $\theta$ . Our result is the posterior distribution  $\mathbb{P}(\theta | \mathcal{D})$ , which combines our beliefs on  $\theta$  based on our prior and the data:

$$\mathbb{P}(\theta | \mathcal{D}) \propto \mathcal{L}(\mathcal{D} | \theta) \cdot \mathbb{P}(\theta). \quad (8)$$

One advantage of Bayesian inference is its ability to accommodate the hierarchical structure of our dataset. For example, suppose that we have  $N$  data points  $\{x_i\}$  which are sampled from some generative model  $\mathcal{P}(\theta)$ . Additionally,

we are given information that each data point belong to one of  $m$  related groups. We can handle this information in three ways.

First, we ignore it and assume that all groups are drawn from the same generative model, i.e.  $x_i \sim \mathcal{P}(\theta)$ . This approach ignores variability across groups.

Second, we assume that the groups are independent from one another and fit a separate  $\theta_j$  for each group, i.e.  $x_i \sim \mathcal{P}(\theta_j)$ . This approach ignores the fact that the groups are related.

The third approach, Bayesian hierarchical modeling, offers a compromise between these two by allowing variation across groups. Here, we assume that each group  $j$  has its own  $\theta_j$  parameter, and  $x_{j[i]} \sim \mathcal{P}(\theta_j)$ , where  $j[i]$  is read as ‘the group data point  $i$  belongs to’. We assume that  $\{\theta_j\}$  are not independent but are samples from a group-level distribution  $\mathcal{Q}$  parametrized by a group-level parameter  $\theta_{group}$ , i.e.  $\theta_j \sim \mathcal{Q}(\theta_{group})$ . Under this hierarchical framework,  $\mathcal{Q}(\theta_{group})$  acts a prior for each parameter  $\theta_j$ . Specifying a prior distribution for  $\theta_{group}$  completes the Bayesian hierarchical model. Our posterior is a joint distribution over each group’s parameter  $\theta_j$  and the group-level parameter  $\theta_{group}$ .

## 2 Additional Material for Main Text Section 3

### 2.1 Complete Table of Notation

In Table 1 we show the full set of notation, BMH model parameters, their interpretation and real-world mapping.

### 2.2 BMH-P Model

**Assumptions.** In Main Text Eqs. (2) and (3) we assume that the item-level features  $\vec{y}^a$  influence the location (i.e. mean) and membership probability of each popularity class  $k$ , while the cascade-level features  $\vec{x}^{ac}$  influence only the membership probability. As a concrete example, if we have two popularity classes (popular and unpopular),  $\mathcal{A}$  being a set of articles,  $\vec{y}^a$  being the headline embedding vector of article  $a$ , and  $\vec{x}^{ac}$  the follower count of the initiator of cascade  $c$ , our assumptions imply how large a cascade will turn out to be (Main Text Eq. (2)) is influenced only by article content  $\vec{y}^a$ , but whether a cascade will be popular or not is influenced by both article content  $\vec{y}^a$  and follower count  $\vec{x}^{ac}$ .

**Likelihood Function.** The log-likelihood of  $\mathcal{P}_\alpha$  given the set of cascade sizes  $\{N_{ac}\}_{ac}$  can be derived as:

$$\begin{aligned}
\mathcal{L}(\mathcal{P}_\alpha | \{N_{ac}\}_{ac}) &= \log \mathbb{P}(\{N_{ac}\}_{ac} | \mathcal{P}_\alpha) \\
&= \log \prod_{a \in \mathcal{A}} \prod_{\mathcal{H}^{ac} \in \mathbb{H}^a} \mathbb{P}(N_{ac} | \mathcal{P}_\alpha) \\
&= \log \prod_{a \in \mathcal{A}} \prod_{\mathcal{H}^{ac} \in \mathbb{H}^a} \mathbb{P}(N_{ac} | \alpha^{ac}) \\
^{(a)} &= \log \prod_{a \in \mathcal{A}} \prod_{\mathcal{H}^{ac} \in \mathbb{H}^a} \mathbb{B}(N_{ac} | \alpha^{ac}) \\
^{(b)} &= \log \prod_{a \in \mathcal{A}} \prod_{\mathcal{H}^{ac} \in \mathbb{H}^a} \sum_{k=1}^{K_\alpha} z_{\alpha,k}^{ac} \cdot \mathbb{B}(N_{ac} | \text{inv-logit}(\delta_{\alpha,k}^a + \vec{\gamma}_{\alpha,k} \cdot \vec{y}^a)) \\
&= \sum_{\mathcal{H}^{ac} \in \mathbb{H}^a, a \in \mathcal{A}} \log \sum_{k=1}^{K_\alpha} z_{\alpha,k}^{ac} \cdot \mathbb{B}(N_{ac} | \text{inv-logit}(\delta_{\alpha,k}^a + \vec{\gamma}_{\alpha,k} \cdot \vec{y}^a)),
\end{aligned}$$

where in (a) we use the fact that the cascade size of a Hawkes process is Borel-distributed with parameter  $\alpha^{ac}$  and in (b) we note that the BMH-P model specifies  $a^{ac}$  as a mixture over the  $K_\alpha$  classes, weighted by the membership probabilities  $\{z_{\alpha,k}^{ac}\}$ .

**Cold-Start Popularity.** First, from our dataset  $\mathcal{A}$ , compute  $\hat{C}_\rho$  as the average cascade count for an article in  $\mathcal{A}$  and  $\hat{f}_\rho(\vec{x}^{ac} | \vec{y}^a)$  as the empirical probability density of the cascade feature vector  $\vec{x}^{ac}$  given item feature vector  $\vec{y}^a$ .

Second, from Main Text Eq. (4) we draw the parameter set  $\vec{p}_{\alpha^*}^{a^*}$  for the out-of-sample item  $a^*$ . Consider an arbitrary cascade  $c$  of item  $a^*$  with feature vector  $\vec{x}^{a^*c}$ . The expected cascade size of  $c$  is given by the expectation of Main Text Eq. (2) over the  $K_\alpha$  popularity classes  $\mathbb{E}_{z_{\alpha,k}^{a^*c}}[\mathbb{E}[N^{a^*c} | \vec{x}^{a^*c}, \vec{y}^{a^*}]]$ . Since  $c$  is arbitrary, we need to average  $\vec{x}^{a^*c}$  out. Hence, our expected cascade size is  $\mathbb{E}_{\vec{x}^{a^*c}} \mathbb{E}_{z_{\alpha,k}^{a^*c}}[\mathbb{E}[N^{a^*c} | \vec{x}^{a^*c}, \vec{y}^{a^*}]]$ . Our estimate  $\hat{N}^{a^*}$  of item  $a^*$ 's popularity is then given by

$$\begin{aligned}
\hat{N}^{a^*} &= \hat{C}_\rho \cdot \mathbb{E}_{\vec{x}^{a^*c}} \mathbb{E}_{z_{\alpha,k}^{a^*c}} [\mathbb{E}[N^{a^*c} | \vec{x}^{a^*c}, \vec{y}^{a^*}]] \\
&= \hat{C}_\rho \cdot \mathbb{E}_{\vec{x}^{a^*c}} \mathbb{E}_{z_{\alpha,k}^{a^*c}} [\text{logit}(\alpha^{a^*c}) | \vec{x}^{a^*c}, \vec{y}^{a^*}] \\
^{(a)} &= \hat{C}_\rho \cdot \mathbb{E}_{\vec{x}^{a^*c}} \sum_{k=1}^{K_\alpha} z_{\alpha,k}^{a^*,c} \cdot \left( \delta_{\alpha,k}^{a^*} + \vec{\gamma}_{\alpha,k} \cdot \vec{y}^{a^*} \right) \\
^{(b)} &= \hat{C}_\rho \cdot \int \sum_{k=1}^{K_\alpha} z_{\alpha,k}^{a^*,c} \cdot \left( \delta_{\alpha,k}^{a^*} + \vec{\gamma}_{\alpha,k} \cdot \vec{y}^{a^*} \right) \cdot f_\rho(\vec{x}^{a^*c} | \vec{y}^{a^*}) \cdot d\vec{x}^{a^*c} \\
^{(c)} &\approx \hat{C}_\rho \cdot \int \sum_{k=1}^{K_\alpha} z_{\alpha,k}^{a^*,c} \cdot \left( \delta_{\alpha,k}^{a^*} + \vec{\gamma}_{\alpha,k} \cdot \vec{y}^{a^*} \right) \cdot \hat{f}_\rho(\vec{x}^{a^*c}) \cdot d\vec{x}^{a^*c},
\end{aligned}$$

where in (a) we use the fact that the BMH-P model specifies  $a^{ac}$  as a mixture over the  $K_\alpha$  classes, weighted by the membership probabilities  $\{z_{\alpha,k}^{ac}\}$ , in (b) we marginalize over the unobserved cascade-level features  $\vec{x}^{a^*c}$  in a cold-start setup, and in (c) we use the simplification  $f_\rho(\vec{x}^{ac}|\vec{y}^a) \approx \hat{f}_\rho(x)$  as detailed in the main text.

To simplify this expression, we impose two additional assumptions on the feature vectors. First, assume our cascade feature vector is one-dimensional, discrete and nonnegative (for instance, this may be the follower count of the seed user). This simplifies our probability density  $\hat{f}_\rho(\vec{x}^{ac}|\vec{y}^a)$  into a probability mass function over  $x \in \mathbb{N} \cup \{0\}$ , converting the integral over  $\vec{x}^{ac}$  into a sum. Second, in practice we usually will not have enough variance across  $\vec{y}^a$  to build  $\hat{f}_\rho(\vec{x}^{ac}|\vec{y}^a)$  reliably, and so we assume that  $\vec{x}^{ac}$  is independent of  $\vec{y}^a$ . These two assumptions allow us to write  $\hat{f}_\rho(\vec{x}^{ac}|\vec{y}^a) \approx \hat{f}_\rho(x)$ . Our expression simplifies to

$$\hat{N}^{a^*} \approx \hat{C}_\rho \cdot \sum_{x=0}^{\infty} \sum_{k=1}^{K_\alpha} z_{\alpha,k}^{a^*,c} \cdot \left( \delta_{\alpha,k}^{a^*} + \vec{\gamma}_{\alpha,k} \cdot \vec{y}^{a^*} \right) \cdot \hat{f}_\rho(x), \quad (9)$$

### 2.3 BMH-K Model

**Assumptions.** In Main Text Eqs. (6) and (7), we assume that the item-level features  $\vec{y}^a$  influence the location of  $\theta^{ac}$  and not  $d^{ac}$ . We found that including influence of item-level features  $\vec{y}^a$  on both parameters leads to identifiability issues in the BMH-K model. We assume  $\vec{y}^a$  influence the location (i.e. mean) and membership probability of each popularity class  $k$ , while the cascade-level features  $\vec{x}^{ac}$  influence only the membership probability. As a concrete example, if we have two kernel classes (slow and fast),  $\mathcal{A}$  being a set of articles,  $\vec{y}^a$  being the headline embedding vector of article  $a$ , and  $\vec{x}^{ac}$  the follower count of the initiator of cascade  $c$ , our assumptions imply the speed at which a cascade will diffuse (Main Text Eq. (6)) is influenced only by article content  $\vec{y}^a$ , but whether a cascade will be slow or fast is influenced by both article content  $\vec{y}^a$  and follower count  $\vec{x}^{ac}$ .

**Likelihood Function.** The log-likelihood of  $\mathcal{P}_\Theta$  given the set of interevent-time distributions  $\{\mathcal{T}^{ac}\}_{ac}$  is

$$\begin{aligned}
\mathcal{L}(\mathcal{P}_\Theta|\{\mathcal{T}^{ac}\}_{ac}) &= \log \mathbb{P}(\{\mathcal{T}^{ac}\}_{ac}|\mathcal{P}_\Theta) \\
&\stackrel{(a)}{=} \log \prod_{\mathcal{H}^{ac} \in \mathbb{H}^a, a \in \mathcal{A}} \left[ \prod_{t_j \in \mathcal{H}^{ac}, j \geq 1} \sum_{t_z < t_j} g(t_j - t_z | \theta^{ac}, d^{ac}) \right] \\
&\stackrel{(b)}{=} \log \prod_{\mathcal{H}^{ac} \in \mathbb{H}^a, a \in \mathcal{A}} f(\mathcal{H}^{ac} | \theta^{ac}, d^{ac}) \\
&\stackrel{(c)}{=} \log \prod_{\mathcal{H}^{ac} \in \mathbb{H}^a, a \in \mathcal{A}} \left[ \sum_{k=1}^{K_\Theta} z_{\Theta,k}^{ac} \cdot f(\mathcal{H}^{ac} | e^{\delta_{\theta,k}^a + \vec{\gamma}_{\theta,k} \cdot \vec{y}^a}, e^{\delta_{d,k}^a}) \right] \\
&= \sum_{\mathcal{H}^{ac} \in \mathbb{H}^a, a \in \mathcal{A}} \log \sum_{k=1}^{K_\Theta} z_{\Theta,k}^{ac} \cdot f(\mathcal{H}^{ac} | e^{\delta_{\theta,k}^a + \vec{\gamma}_{\theta,k} \cdot \vec{y}^a}, e^{\delta_{d,k}^a}),
\end{aligned}$$

where in (a) we make use of the likelihood for the interevent-time distribution for separable Hawkes processes as derived in [2], in (b) we set  $f(\mathcal{H}|\theta, d) = \prod_{t_j \in \mathcal{H}} \sum_{t_z < t_j} g(t_j - t_z | \theta, d)$ , and in (c) we use the fact that the BMH-K model specifies  $\Theta^{ac}$  as a mixture over the  $K_\Theta$  classes, weighted by the membership probabilities  $\{z_{\Theta,k}^{ac}\}$ .

**Half-Life Prediction.** Under the BMH-K model, the half-life of an out-of-sample item  $a^*$  can be expressed as

$$\begin{aligned}
\hat{\tau}_{1/2}^{a^*} &= \mathbb{E}_{\vec{x}^{a^*c}} \mathbb{E}_{z_{\Theta,k}^{a^*c}} \left[ \tau_{1/2}^{a^*} | \vec{x}^{a^*c}, \vec{y}^{a^*} \right] \\
&\stackrel{(a)}{=} \mathbb{E}_{\vec{x}^{a^*c}} \mathbb{E}_{z_{\Theta,k}^{a^*c}} \left[ d^{a^*c} \cdot (2^{\theta^{a^*c}} - 1) | \vec{x}^{a^*c}, \vec{y}^{a^*} \right] \\
&\stackrel{(b)}{=} \mathbb{E}_{\vec{x}^{a^*c}} \sum_{k=1}^{K_\Theta} z_{\Theta,k}^{a^*,c} \cdot e^{\delta_{d,k}^{a^*}} \cdot \left[ 2^{\exp(\delta_{\theta,k}^{a^*} + \vec{\gamma}_{\theta,k} \cdot \vec{y}^{a^*})} - 1 \right] \\
&\stackrel{(c)}{\approx} \sum_{x=0}^{\infty} \sum_{k=1}^{K_\Theta} z_{\Theta,k}^{a^*,c} \cdot e^{\delta_{d,k}^{a^*}} \cdot \left[ 2^{\exp(\delta_{\theta,k}^{a^*} + \vec{\gamma}_{\theta,k} \cdot \vec{y}^{a^*})} - 1 \right] \cdot \hat{f}_\rho(x),
\end{aligned}$$

where in (a) we use the expression for the half-life of a Hawkes process under the power law  $g(t) = \theta \cdot d^\theta \cdot (t+d)^{-(1+\theta)}$  (i.e. by solving  $\tau_{1/2}$  such that  $\int_0^{\tau_{1/2}} g(t)dt = \frac{1}{2}$ ), in (b) we use the fact that the BMH-K model specifies  $\Theta^{ac}$  as a mixture over the  $K_\Theta$  classes, weighted by the membership probabilities  $\{z_{\Theta,k}^{ac}\}$ , and in (c) we marginalize over the unobserved cascade-level features  $\vec{x}^{a^*c}$  and use the simplification  $f_\rho(\vec{x}^{ac}|\vec{y}^a) \approx \hat{f}_\rho(x)$  as detailed in the main text.

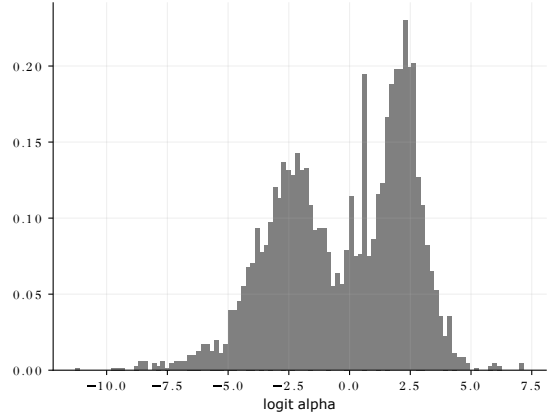

Fig. 1: Distribution of DMM-estimated  $\text{logit}(\alpha)$  across *RNIX* publishers. We note the bimodality of the distribution, with the modes corresponding to low and high cascade sizes. Based on this observation we set  $K_\alpha = 2$  for the BMH-P model.

### 3 Additional Material for Main Text Section 4

#### 3.1 Selection of $K_\alpha$ and $K_\Theta$

To guide the selection of the number of mixture components for the BMH-P (i.e.  $K_\alpha$ ) and BMH-K (i.e.  $K_\Theta$ ) models in Main Text Section 4, we fit the DMM [2] to each publisher in *RNIX*. Given that the EM algorithm is very sensitive to initial conditions, we use 10 random EM initializations and select the output that yields the highest log-likelihood.

We collect the distribution of parameter estimates for  $\text{logit}(\alpha)$  across publishers in Fig. 1. We see two modes for  $\alpha$ , corresponding to cascade groups with low and high sizes, prompting us to set  $K_\alpha = 2$  in Main Text Section 4.

We collect the distribution of parameter estimates for  $(\log(c), \log(\theta))$  across publishers in the upper plot of Fig. 2, where we see three modes for the kernel parameters. From the lower plot of Fig. 2, we can interpret these modes as belonging to usual, fast and slow cascade groups, prompting us to set  $K_\Theta = 3$  in Main Text Section 4.

#### 3.2 Prior Specification for the BMH-P Model

The full set of priors for the BMH-P model implementation is given below. Informative priors are set for  $\delta_{\alpha,1}, \delta_{\alpha,2}, \delta_{z_{\alpha,2}}$  based on the observations in Section 3.1. Weakly informative priors are set for the other parameters. We use a Laplace prior on  $\vec{\gamma}_{\alpha,1}, \vec{\gamma}_{\alpha,2}, \vec{\gamma}_{z_{\alpha,2}}$  to impose regularization given the high dimensionality of the article feature vector ( $|\vec{y}^a| = 32$ ) we consider.

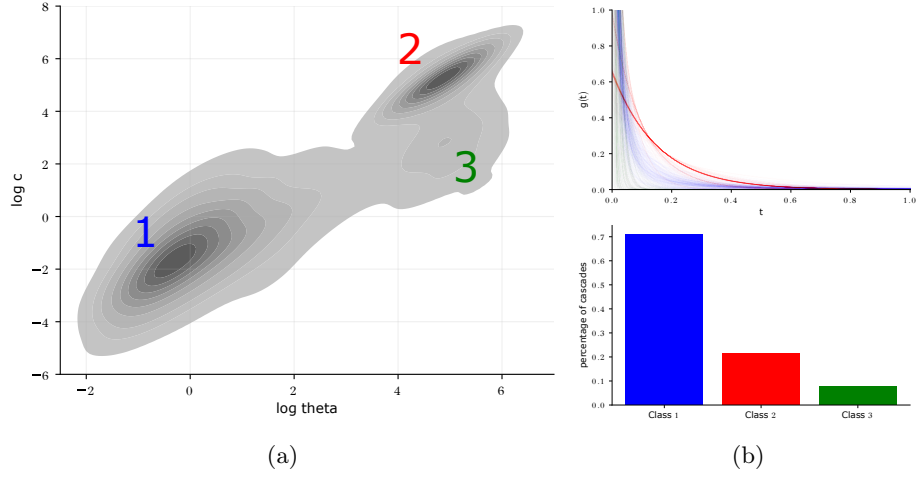

Fig. 2: (a) Distribution of DMM-estimated  $(\log(c), \log(\theta))$  across *RNIX* publishers. We observe the trimodality of the distribution, with the modes corresponding to usual (labeled 1), slow (labeled 2) and fast (labeled 3) cascades. Based on this observation we set  $K_{\Theta} = 3$  for the BMH-K model. (b) In the top plot, we show samples of the power law kernel  $g$  for the three classes. In the bottom plot, we show the distribution of cascades for each class.

$$\begin{aligned}
\delta_{\alpha,1} &\sim \mathcal{N}(-2, 0.5) \\
\delta_{\alpha,2} &\sim \mathcal{N}(2, 0.5) \\
\delta_{z_{\alpha,2}} &\sim \mathcal{N}(-1.39, 0.5) \\
\vec{\beta}_{z_{\alpha,2}} &\sim \mathcal{N}(0, 0.1) \\
\vec{\gamma}_{\alpha,1}, \vec{\gamma}_{\alpha,2}, \vec{\gamma}_{z_{\alpha,2}} &\sim \text{Laplace}(0, 0.01) \\
\Omega_{\alpha} &\sim \text{LKJCorr}(2) \\
\sigma_{\delta_{\alpha,1}}, \sigma_{\delta_{\alpha,2}}, \sigma_{\delta_{z_{\alpha,2}}} &\sim \mathcal{N}(0, 1) \\
\sigma_{\vec{\beta}_{z_{\alpha,2}}} &\sim \mathcal{N}(0, 0.1)
\end{aligned}$$

### 3.3 Prior Specification for the BMH-K Model

The full set of priors for the BMH-K model implementation is given below. Informative priors are set for  $\delta_{\theta,1}, \delta_{d,1}, \delta_{\theta,2}, \delta_{d,2}, \delta_{\theta,3}, \delta_{d,3}, \delta_{z_{\Theta,2}}, \delta_{z_{\Theta,3}}$  based on the observations in Section 3.1. Weakly informative priors are set for the other parameters. We use a Laplace prior on  $\vec{\gamma}_{\Theta,2}, \vec{\gamma}_{\Theta,3}, \vec{\gamma}_{z_{\Theta,2}}, \vec{\gamma}_{z_{\Theta,3}}$  to impose regularization given the high dimensionality of the article feature vector ( $|\vec{y}^a| = 32$ ) we

consider. For  $\Omega_{\boldsymbol{\theta},1}, \Omega_{\boldsymbol{\theta},2}, \Omega_{\boldsymbol{\theta},3}$ , we set a LKJCorr(0.5) prior (i.e. higher weights on the tails of  $[0,1]$ ) as  $(\theta, d)$  for any given Hawkes fit are correlated.

$$\begin{aligned}
\delta_{\theta,1} &\sim \mathcal{N}(-0.41, 0.5) \\
\delta_{d,1} &\sim \mathcal{N}(-1.37, 1) \\
\delta_{\theta,2} &\sim \mathcal{N}(4, 0.5) \\
\delta_{d,2} &\sim \mathcal{N}(4.805, 0.5) \\
\delta_{\theta,3} &\sim \mathcal{N}(4, 0.5) \\
\delta_{d,3} &\sim \mathcal{N}(1, 0.5) \\
\delta_{z_{\boldsymbol{\theta},2}}, \delta_{z_{\boldsymbol{\theta},3}} &\sim \mathcal{N}(-2, 1) \\
\vec{\beta}_{z_{\boldsymbol{\theta},2}}, \vec{\beta}_{z_{\boldsymbol{\theta},3}} &\sim \mathcal{N}(0, 0.1) \\
\vec{\gamma}_{\boldsymbol{\theta},2}, \vec{\gamma}_{\boldsymbol{\theta},3}, \vec{\gamma}_{z_{\boldsymbol{\theta},2}}, \vec{\gamma}_{z_{\boldsymbol{\theta},3}} &\sim \text{Laplace}(0, 0.01) \\
\Omega_{\boldsymbol{\theta},1}, \Omega_{\boldsymbol{\theta},2}, \Omega_{\boldsymbol{\theta},3} &\sim \text{LKJCorr}(0.5) \\
\Omega_{z_{\boldsymbol{\theta}}} &\sim \text{LKJCorr}(2) \\
\sigma_{\delta_{\theta,1}}, \sigma_{\delta_{\theta,2}}, \sigma_{\delta_{\theta,3}}, \sigma_{\delta_{d,1}}, \sigma_{\delta_{d,2}}, \sigma_{\delta_{d,3}}, \sigma_{\delta_{z_{\boldsymbol{\theta},2}}}, \sigma_{\delta_{z_{\boldsymbol{\theta},3}}} &\sim \mathcal{N}(0, 1) \\
\sigma_{\vec{\beta}_{z_{\boldsymbol{\theta},2}}}, \sigma_{\vec{\beta}_{z_{\boldsymbol{\theta},3}}} &\sim \mathcal{N}(0, 0.1)
\end{aligned}$$

### 3.4 Implementation Details.

We use the Python implementation of Stan [1] to run both the BMH-P and BMH-K models. We run for 4 chains, adapt delta set to 0.9, 500 warmup iterations and 500 post-warmup iterations. To speed up convergence we implement non-centered parametrization [3] for each of the normally distributed priors.

## 4 Additional Material for Main Text Section 5

### 4.1 Performance Heatmaps for CNIX and RNIX

We show performance heatmaps for a selection of CNIX publishers in Fig. 3 and RNIX publishers in Fig. 4. Note the different patterns of which headline style works for each publisher, implying that the BMH model picks up subtle differences of what is effective across publishers.

## References

1. Carpenter, B., Gelman, A., Hoffman, M.D., Lee, D., Goodrich, B., Betancourt, M., Brubaker, M., Guo, J., Li, P., Riddell, A.: Stan: A probabilistic programming language. *Journal of statistical software* **76**(1) (2017)

2. Kong, Q., Rizoïu, M.A., Xie, L.: Describing and predicting online items with reshare cascades via dual mixture self-exciting processes. In: Proceedings of the 29th ACM International Conference on Information & Knowledge Management. pp. 645–654 (2020)
3. Papaspiliopoulos, O., Roberts, G.O., Sköld, M.: A general framework for the parametrization of hierarchical models. *Statistical Science* pp. 59–73 (2007)
4. Tomasi, C.: Estimating gaussian mixture densities with em—a tutorial. *Duke University* pp. 1–8 (2004)

Table 1: Table of Notation.

| Parameter                                                   | Interpretation                                                        | Real-World Mapping                  |
|-------------------------------------------------------------|-----------------------------------------------------------------------|-------------------------------------|
| <i>Source-Level</i>                                         |                                                                       |                                     |
| $\rho$                                                      | source of items                                                       | news publisher                      |
| $\mathcal{A}$                                               | set of items produced by $\rho$                                       | news articles from publisher $\rho$ |
| $f_\rho(\cdot)$                                             | follower count distribution                                           |                                     |
| $\hat{C}_\rho$                                              | cascade count estimate                                                |                                     |
| <i>Item-Level</i>                                           |                                                                       |                                     |
| $a \in \mathcal{A}$                                         | item produced by $\rho$                                               | news article                        |
| $\mathbb{H}^a$                                              | set of cascades related to item $a$                                   | retweet cascades for article $a$    |
| $\vec{y}^a$                                                 | item-level features                                                   | headline embedding for article $a$  |
| $N^a$                                                       | item popularity                                                       | overall tweet count for article $a$ |
| $\tau_{1/2}^a$                                              | content half-life                                                     |                                     |
| <i>Cascade-Level</i>                                        |                                                                       |                                     |
| $\mathcal{H}^{ac} \in \mathbb{H}^a$                         | cascade related to item $a$                                           | retweet cascade for article $a$     |
| $\vec{x}^{ac}$                                              | cascade-level features                                                | follower count of seed user         |
| $N^{ac}$                                                    | cascade size                                                          |                                     |
| $\tau_{1/2}^{ac}$                                           | cascade half-life                                                     |                                     |
| $\mathcal{T}^{ac}$                                          | interevent-time distribution                                          |                                     |
| $\alpha^{ac}$                                               | Hawkes branching factor                                               |                                     |
| $\Theta^{ac}$                                               | Hawkes kernel parameters                                              |                                     |
| <i>BMH-P</i>                                                |                                                                       |                                     |
| $K_\alpha$                                                  | # of BMH-P mixture classes                                            |                                     |
| $\vec{\gamma}_{\alpha,k}$                                   | effect of $\vec{y}^a$ on center of class $k$                          |                                     |
| $\vec{\gamma}_{z_{\alpha,k}}$                               | effect of $\vec{y}^a$ on membership probability of class $k$          |                                     |
| $\delta_{\alpha,k}^a / \delta_{\alpha,k}$                   | item-/ publisher-level baseline value of $\log(\alpha)$ for class $k$ |                                     |
| $\vec{\beta}_{\alpha,k}^a / \vec{\beta}_{\alpha,k}$         | effect of $\vec{x}^{ac}$ on center of class $k$                       |                                     |
| $z_{\alpha,k}^{ac}$                                         | mem. probability for class $k$                                        |                                     |
| $\delta_{z_{\alpha,k}}^a / \delta_{z_{\alpha,k}}$           | item-/ publisher-level mem. prob. softmax baseline for class $k$      |                                     |
| $\vec{\beta}_{z_{\alpha,k}}^a / \vec{\beta}_{z_{\alpha,k}}$ | effect of $\vec{x}^{ac}$ on membership probability for class $k$      |                                     |
| $\vec{p}_\alpha^a / \vec{p}_\alpha$                         | item-/ pub.-level parameter vector                                    |                                     |
| $\Sigma_\alpha / \Omega_\alpha$                             | cov./ corr. matrix for $\vec{p}_\alpha$                               |                                     |
| <i>BMH-K</i>                                                |                                                                       |                                     |
| $K_\Theta$                                                  | # of BMH-K mixture classes                                            |                                     |
| $\vec{\gamma}_{\theta,k}$                                   | effect of $\vec{y}^a$ on center of class $k$                          |                                     |
| $\vec{\gamma}_{z_{\Theta,k}}$                               | effect of $\vec{y}^a$ on membership probability of class $k$          |                                     |
| $\delta_{\theta,k}^a / \delta_{\theta,k}$                   | item-/ publisher-level baseline value of $\log(\theta)$ for class $k$ |                                     |
| $\vec{\beta}_{\theta,k}^a / \vec{\beta}_{\theta,k}$         | effect of $\vec{x}^{ac}$ on center of class $k$                       |                                     |
| $z_{\Theta,k}^{ac}$                                         | mem. probability for class $k$                                        |                                     |
| $\delta_{z_{\Theta,k}}^a / \delta_{z_{\Theta,k}}$           | item-/ publisher-level mem. prob. softmax baseline for class $k$      |                                     |
| $\vec{\beta}_{z_{\Theta,k}}^a / \vec{\beta}_{z_{\Theta,k}}$ | effect of $\vec{x}^{ac}$ on membership probability for class $k$      |                                     |
| $\vec{p}_{\Theta,k}^a / \vec{p}_{\Theta,k}$                 | item-/ pub.-level kernel parameter baseline values for class $k$      |                                     |
| $\vec{p}_{z_{\Theta}}^a / \vec{p}_{z_{\Theta}}$             | item-/ pub.-level membership probability parameters for class $k$     |                                     |
| $\Sigma_{\Theta,k} / \Omega_{\Theta,k}$                     | cov./ corr. matrix for $\vec{p}_{\Theta,k}$                           |                                     |
| $\Sigma_{z_{\Theta}} / \Omega_{z_{\Theta}}$                 | cov./ corr. matrix for $\vec{p}_{z_{\Theta}}$                         |                                     |

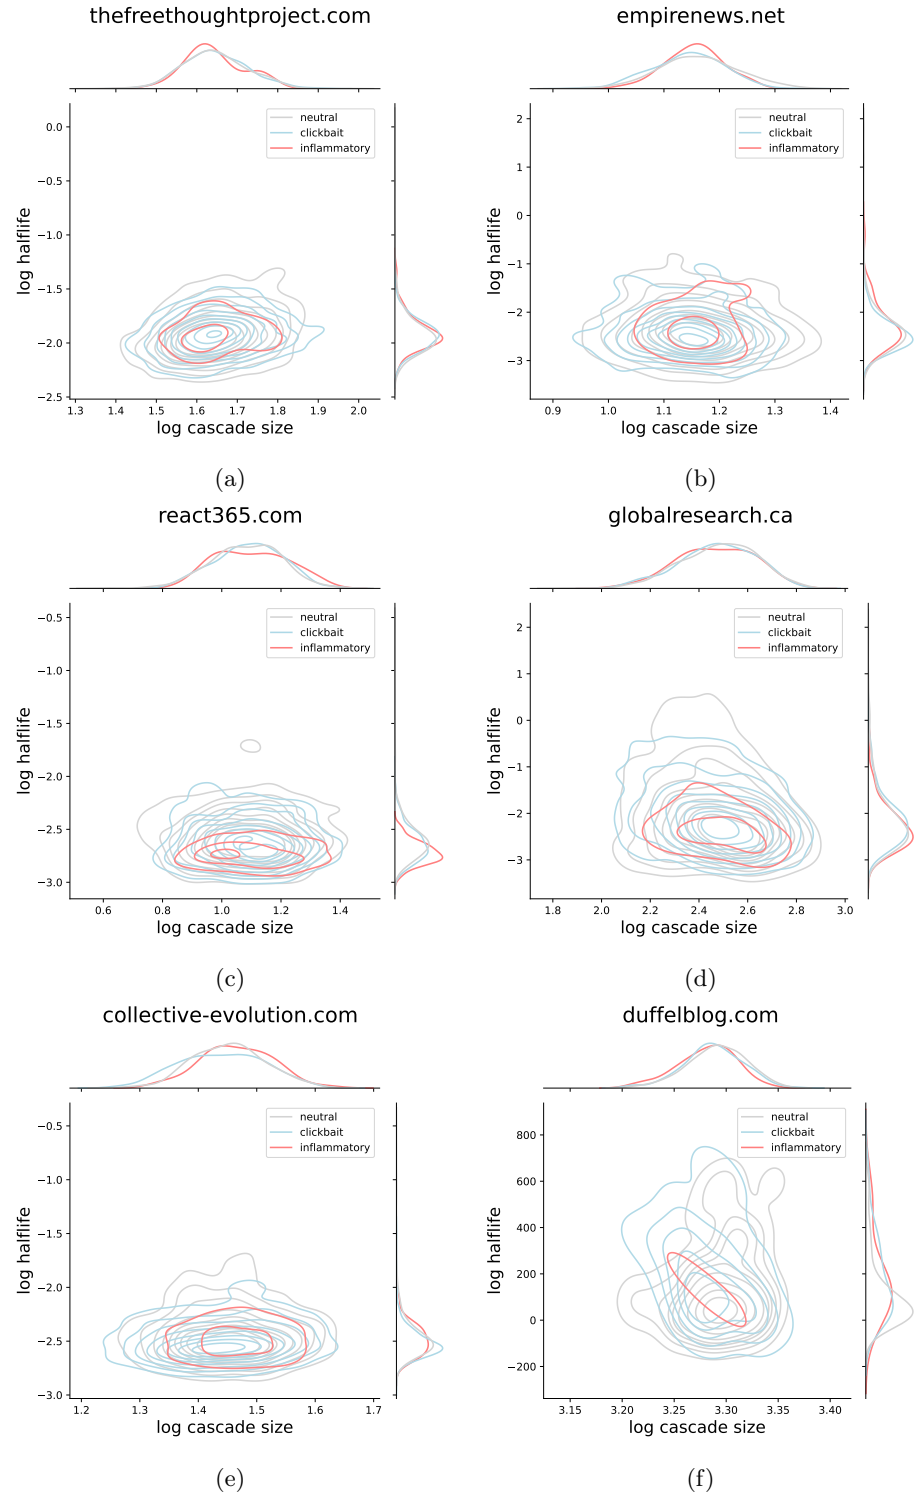

Fig. 3: Performance heatmaps for a selection of CNIX publishers.

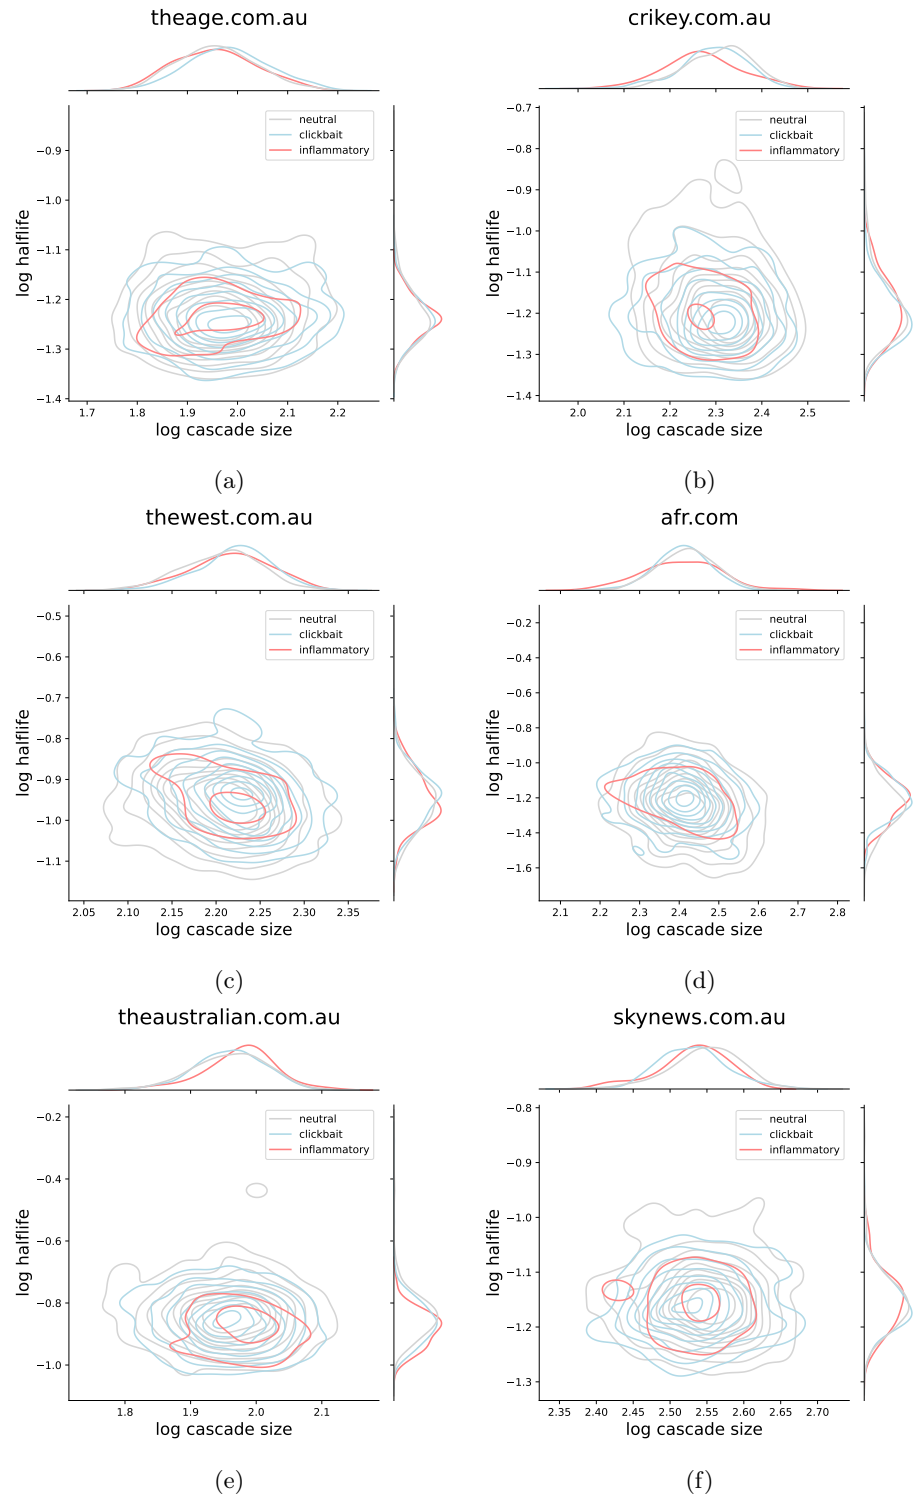

Fig. 4: Performance heatmaps for a selection of RNIX publishers.
